# Supplementary material for: Why We Feel: Breaking Boundaries in Emotional Reasoning with Multimodal Large Language Models
Source: arXiv:2504.07521 source file (2025-04-17)
Supplement: Supplementary file 1 [file datasheet.tex]

\section{Datasheet}
\subsection{Motivation}
\begin{enumerate}
    \item \textbf{For what purpose was the dataset created?} \textit{Our benchmark dataset was created to enhance the emotion comprehension abilities of the emotion-related deep learning models. And it can be used as a benchmark for VLLM's emotional knowledge assessment.}
    \item \textbf{Who created the dataset and on behalf of which entity?} \textit{The dataset was developed by a consortium of scientists in affect computing and multimedia.}
    \item \textbf{Who funded the creation of the dataset?} \textit{The main funding body is the National Natural Science Foundation of China. Other funding sources of individual authors are listed in the acknowledgment section of the main manuscript.}
\end{enumerate}

\subsection{Distribution}
\begin{enumerate}
    \item \textbf{Will the dataset be distributed to third parties outside of the entity (e.g., company, institution, organization) on behalf of which the dataset was created?} \textit{Yes, the dataset is open to the public.}
    \item \textbf{How will the dataset will be distributed (e.g., tarball on website, API, GitHub)?} \textit{The dataset and the code used for developing baseline models will be distributed through GitHub.}
    \item \textbf{Have any third parties imposed IP-based or other restrictions on the data associated with the instances?} \textit{We refine the dataset from CAER-S~\cite{caer-s} and EmoSet~\cite{yang2023emoset}, users should follow their open source license.}
    \item \textbf{Do any export controls or other regulatory restrictions apply to the dataset or to individual instances?} \textit{No.}
\end{enumerate}

\subsection{Maintenance}
\begin{enumerate}
    \item \textbf{Who will be supporting/hosting/maintaining the dataset?} \textit{Shenzhen Technology University Multimodal Intelligent Perception System Lab (MIPS-Lab) will support, host and maintain the dataset.}
    \item \textbf{How can the owner/curator/manager of the dataset be contacted (e.g., email address)?} \textit{The owner/curator/manager(s) of the dataset can be contacted through following emails: Yuxiang Lin (lin.yuxiang.contact@gmail.com), Xiaojiang Peng (pengxiaojiang@sztu.edu.cn), Jun-Yan He (junyanhe1989@gmail.com) and Zhi-Qi Cheng (zhiqic@cs.cmu.edu).}
    \item \textbf{Is there an erratum?} \textit{No. If errors are found in the future, we will release errata on the GitHub page for the dataset (https://github.com/Lum1104/EmCoBench).}
    \item \textbf{Will the dataset be updated (e.g., to correct labeling errors, add new instances, delete instances)?} \textit{Yes, the datasets will be updated whenever necessary to ensure accuracy, and announcements will be made accordingly. These updates will be posted on the GitHub page for the dataset (https://github.com/Lum1104/EmCoBench).}
    \item \textbf{If the dataset relates to people, are there applicable limits on the retention of the data associated with the instances (e.g., were the individuals in question told that their data would be retained for a fixed period of time and then deleted?)} \textit{N/A. We refine the dataset from CAER-S~\cite{caer-s} and EmoSet~\cite{yang2023emoset}.}
    \item \textbf{Will older version of the dataset continue to be supported/hosted/maintained?} \textit{Yes, older versions of the dataset will continue to be maintained and hosted.}
    \item \textbf{If others want to extend/augment/build on/contribute to the dataset, is there a mechanisms for them to do so?} \textit{We appreciate the community in extending our dataset. Simply open a pull request on the GitHub page and we will review it regularly.}
\end{enumerate}

\subsection{Composition}
\begin{enumerate}
    \item \textbf{What do the instance that comprise the dataset represent (e.g., documents, photos, people, countries?)} \textit{Each instance includes an image-question-triggers pair. The image depicts humans displaying emotions, accompanied by a corresponding question and identified emotional triggers.}
    \item \textbf{How many instances are there in total (of each type, if appropriate)?} \textit{The basic EmCoBench consists of 1,615 instances encompassing 78 fine-grained emotion types. Additionally, the multifaceted complex EmCoBench comprises 50 instances.}
    \item \textbf{Does the dataset contain all possible instances or is it a sample of instances from a larger set?} \textit{Yes, EmCoBench is refined from CAER-S~\cite{caer-s} and EmoSet~\cite{yang2023emoset}, and it has undergone thorough human annotation for emotional triggers.}
    \item \textbf{Is there a label or target associated with each instance?} \textit{Yes, each instance includes both input and target (ground truth label) variables.}
    \item \textbf{Is any information missing from individual instances?} \textit{No.}
    \item \textbf{Are there recommended data splits (e.g., training, development/validation, testing)?} \textit{The EmCoBench is a test-only benchmark, all dataset should be used in testing.}
    \item \textbf{Are there any errors, sources of noise, or redundancies in the dataset?} \textit{No.}
    \item \textbf{Is the dataset self-contained, or does it link to or otherwise rely on external resources (e.g., websites, tweets, other datasets)?} \textit{Yes, CAER-S~\cite{caer-s} and EmoSet~\cite{yang2023emoset} can be downloaded from https://caer-dataset.github.io/ and https://vcc.tech/EmoSet~\cite{yang2023emoset} respectively.}
    \item \textbf{Does the dataset contain data that might be considered confidential?} \textit{No.}
    \item \textbf{Does the dataset contain data that, if viewed directly, might be offensive, insulting, threatening, or might otherwise cause anxiety?} \textit{No.}
\end{enumerate}

\subsection{Collection Process}
\begin{enumerate}
    \item \textbf{How was the data associated with each instance acquired?} \textit{The data associated with a VLLM-assisted dataset annotation method CFSA.} References for CFSA are provided in the main manuscript.
    \item \textbf{What mechanisms or procedures were used to collect the data (e.g., hardware apparatus or sensor, manual human curation, software program, software API)?} \textit{We used 8 cards NVIDIA A100 GPU to run the CFSA methods, together with a comprehensive manual review annotation.}
    \item \textbf{Who was involved in the data collection process (e.g., students, crowdworkers, contractors) and how were they compensated (e.g., how much were crowdworkers paid)?} \textit{Students at Shenzhen Technology University, and Shenzhen Institute of Advanced Technology, CAS were involved in the data annotation process. No crowdworkers were involoved during the data annotation process.}
    \item \textbf{Does the dataset relate to people?} \textit{Yes, this dataset is about general human emotion comprehension.}
    \item \textbf{Did you collect the data from the individuals in questions directly, or obtain it via third parties or other sources (e.g., websites)?} \textit{We refine the dataset from CAER-S~\cite{caer-s} and EmoSet~\cite{yang2023emoset}.}
\end{enumerate}

\subsection{Uses}
\begin{enumerate}
    \item \textbf{Has the dataset been used for any tasks already?} \textit{No, this dataset has not been used for any tasks yet.}
    \item \textbf{What (other) tasks could be the dataset be used for?} Please refer to the Section~\ref{supp:application} for other applications.
    \item \textbf{Is there anything about the composition of the dataset or the way it was collected and preprocessed/cleaned/labeled that might impact future uses?} \textit{No.}
    \item \textbf{Are there tasks for which the dataset should not be used?} \textit{No.}
\end{enumerate}
