# Supplementary material for: Why We Feel: Breaking Boundaries in Emotional Reasoning with Multimodal Large Language Models
Source: arXiv:2504.07521 source file (2025-04-17)
Supplement: Supplementary file 2 [file evaluate_metrics.tex]

\section{Evaluation Metrics}
Given the subjective nature of emotions, multiple triggers could elicit a particular response. Despite thorough reviews, some triggers may be missed. Therefore, we use Recall as the evaluation metric. If the model's understanding overlaps with our ground truth, it is considered correct. Formally, recall is calculated as:

\begin{equation}
\label{metric}
\text{Recall} = \frac{TP}{TP + FN}
\end{equation}

An emotional trigger identified by the model is considered a true positive $TP$ if it overlaps with any part of our ground truth annotations, otherwise considered as false negatives $FN$. We implemented this using LLaMA-3 and ChatGPT-3.5 (gpt-3.5-turbo-0125) to input emotion comprehension results from various VLLMs and identify overlaps with the ground truth for metric calculations.
\paragraph{Emotional Trigger Recall.}
Given the subjective nature of emotions, multiple triggers could elicit a particular response, and some may be missed despite thorough reviews. Therefore, we use Recall as the evaluation metric. If the model's understanding overlaps with our ground truth, it is considered correct. An emotional trigger identified by the model is a true positive if it overlaps with any part of our ground truth annotations; otherwise, it is a false negative. We implemented this using LLaMA-3 and ChatGPT-3.5 (gpt-3.5-turbo-0125) to input emotion comprehension results from various VLLMs and identify overlaps for metric calculations.

\paragraph{Long-term Coherence.}
Long-term coherence in the context of emotion comprehension evaluates a model's ability to maintain consistent emotional and thematic understanding throughout extended text. This metric is crucial for tasks where the emotional narrative or flow must remain logical and coherent over multiple sentences or paragraphs. We implement this metric using BERT~\cite{devlin2018bert} embeddings to measure semantic similarity between adjacent sentences or paragraphs.
